# Supplementary material for: Design of conditions for emergence of self-replicators
Source: arXiv:1709.09191 ancillary file (2018-11-13)
Supplement: Supplementary file 1 [file SI.pdf]

# Supplementary Information: Design of conditions for self-replication

Sumantra Sarkar* and Jeremy L. England†
*Physics of Living Systems, Massachusetts Institute of Technology,*
*400 Technology Square, Cambridge, MA 02139, USA*

* Center for Nonlinear Studies, Los Alamos National Laboratory, Los Alamos, NM 87544, USA; sumantra@lanl.gov
† jengland@mit.edu

**CONTENTS**


I. Modes of self-replication 3
A. Scheme 1 3
B. Schemes 2 and 3 4
C. Schemes 4 and 5 4

II. Probability of self-replication 5
A. Percolation of autocatalytic cycles with access to food 5
1. Availability of food 6
2. Availability of autocatalytic cycle 6
3. Probability of autocatalytic cycles with access to food 7
B. Probability of side reactions 7
C. Probability of self-replication 8
D. Percolation probabilities and conditions for self-replication 9
E. Asymptotic bound on the probability of self-replication 9

III. Factors affecting probability of self-replication 11

IV. Control of $p_{sr}$ through dimerization reactions 11

V. Probability distribution for specificity 12

References 12

## I. MODES OF SELF-REPLICATION

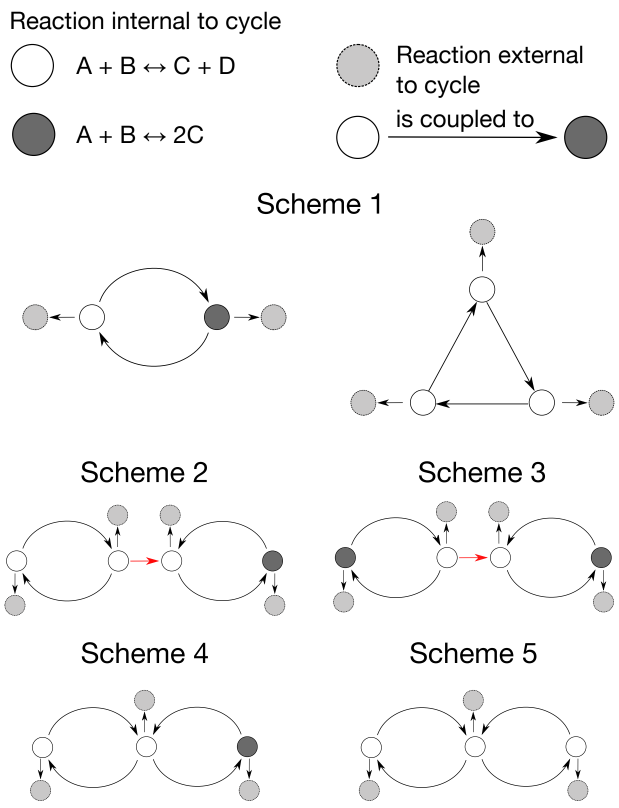


FIG. 1. **Modes of self-replication:** *Scheme 1:* Isolated autocatalytic cycles (ACC). On the left is a two step ACC and on the right is a three step ACC. *Scheme 2:* A catalytic cycle (CC) is coupled to an ACC through the waste product of the former (red arrow). *Scheme 3:* ACC coupled to another ACC through the waste of the former. *Scheme 4:* CC is coupled to ACC through a catalyst, which is also catalyst for the ACC. *Scheme 5:* CC is coupled to another CC by sharing a catalyst molecule between them. In all of these schemes the light gray reactions are reactions that couple to the reactions in a motif, but are not part of it.

### A. Scheme 1

We consider only the two step cycle as it is easier to solve analytically. Numerical investigation shows (not shown here) that the result follows for the three and higher step cycles as well.

Let's consider the following two reactions:

$$X \rightarrow Y \tag{1}$$

$$Y \rightarrow 2X \tag{2}$$

For simplicity we assume that these reactions are completely irreversible and have rate constants 1. We model the effect of parasitic side reactions by annihilation reactions:

$$X \rightarrow \phi \text{ rate constant, } r = k_x \tag{3}$$

$$Y \rightarrow \phi, \text{ rate constant, } r = k_y \tag{4}$$

The jacobian of these chemical system is:

$$J_1 = \begin{bmatrix} -(1+k_x) & 2 \\ 1 & -(1+k_y) \end{bmatrix} \tag{5}$$

One of the eigenvalues of this jacobian has a positive real part if and only if:

$$k_x + k_y + k_x k_y \leq 1 \tag{6}$$

The specificities of the reactions are $\sigma_1 = 1/(1+k_x)$ and $\sigma_2 = 1/(1+k_y)$. Therefore, the cycle specificity is:

$$\sigma = \sigma_1 \times \sigma_2 \tag{7}$$
$$= \frac{1}{1+k_x+k_y+k_xk_y} \tag{8}$$
$$\tag{9}$$

Therefore, for positive eigenvalue, using $k_x+k_y+k_xk_y \leq 1$, we find that $\sigma \geq 0.5$, in agreement with previous results [1, 2].

### B. Schemes 2 and 3

The reactions are as follows.

$$X \rightarrow Y+W, r=1 \tag{10}$$
$$Y \rightarrow \alpha X, r=1 \tag{11}$$
$$W \rightarrow V, r=1 \tag{12}$$
$$V \rightarrow 2W, r=1 \tag{13}$$
$$X \rightarrow \phi, r=k_x \tag{14}$$
$$Y \rightarrow \phi, r=k_y \tag{15}$$
$$W \rightarrow \phi, r=k_w \tag{16}$$
$$V \rightarrow \phi, r=k_v \tag{17}$$

$\alpha = 1$ for scheme 2 and $\alpha = 2$ for scheme 3.

The corresponding Jacobian is:

$$J_2 = \begin{bmatrix} -(1+k_x) & \alpha & 0 & 0 \\ 1 & -(1+k_y) & 0 & 0 \\ 1 & 0 & -(1+k_w) & 2 \\ 0 & 0 & 1 & -(1+k_v) \end{bmatrix} \tag{18}$$

$J_2$ can be solved similar to $J_1$ and the criteria for positive eigenvalues are:

$$k_w+k_v+k_wk_v \leq 1, \text{for schemes 2 and 3, or} \tag{19}$$
$$k_x+k_y+k_xk_y \leq 1, \text{only for scheme 3} \tag{20}$$

Therefore, the criteria for self-replication is same as scheme 1: ACC specificity has to be greater than 0.5.

### C. Schemes 4 and 5

The reactions are as follows.

$$X \rightarrow Y+W, r=1 \tag{21}$$
$$Y \rightarrow X, r=1 \tag{22}$$
$$W \rightarrow \alpha X, r=1 \tag{23}$$
$$X \rightarrow \phi, r=k_x \tag{24}$$
$$Y \rightarrow \phi, r=k_y \tag{25}$$
$$W \rightarrow \phi, r=k_w \tag{26}$$

$\alpha = 2$ for scheme 4 and $\alpha = 1$ for scheme 5.

The corresponding Jacobian is:

$$J_3 = \begin{bmatrix} -(1+k_x) & 1 & \alpha \\ 1 & -(1+k_y) & 0 \\ 1 & 0 & -(1+k_w) \end{bmatrix} \tag{27}$$

The eigenvalues of this jacobian is complicated and finding a criteria akin to the ones for schemes 1-3 is tiresome and impractical. However, the eigenvalues can be found numerically and as a function of $k_{x,y,w}$. In the following figures (Fig. **??**), we list the values of $k_{x,y,w}$ and the corresponding $\sigma_{1,2,3}$ for which the real part of at least one of the eigenvalues is positive. Positive eigenvalue, hence exponential growth, is observed even when the cycle specificities are less than 0.5.

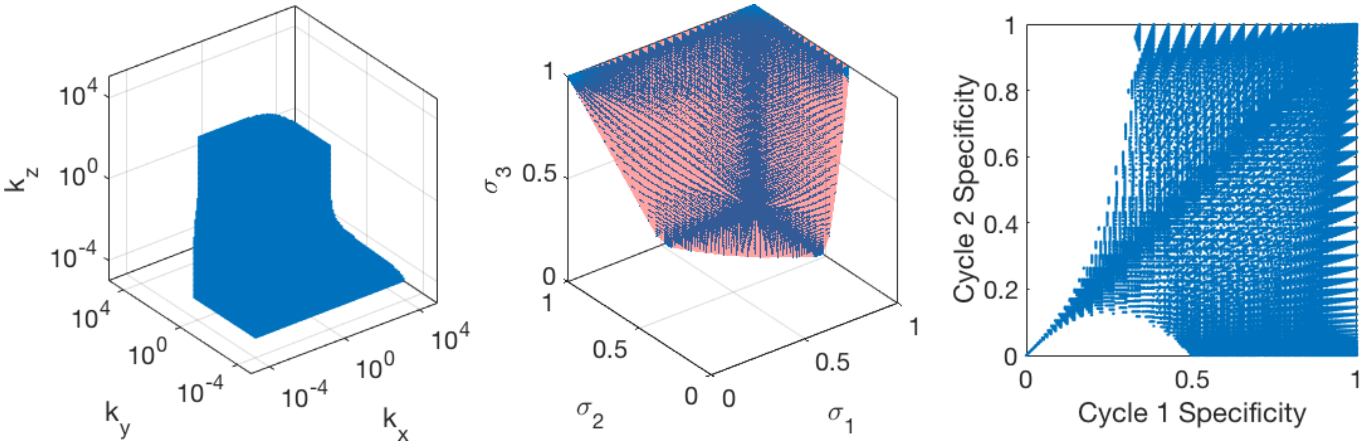


FIG. 2. **Scheme 4:** (a) Scatter plot of $k_{x,y,w}$ values for which real part of at least one eigenvalue is positive. (b) The scatter plot of $\sigma_{1,2,3}$ for which the same condition is true. (c) Scatter plot of cycle specificities of the two coupled cycle for the same condition. Positive eigenvalue is observed even when the cycle specificities are much below 0.5.

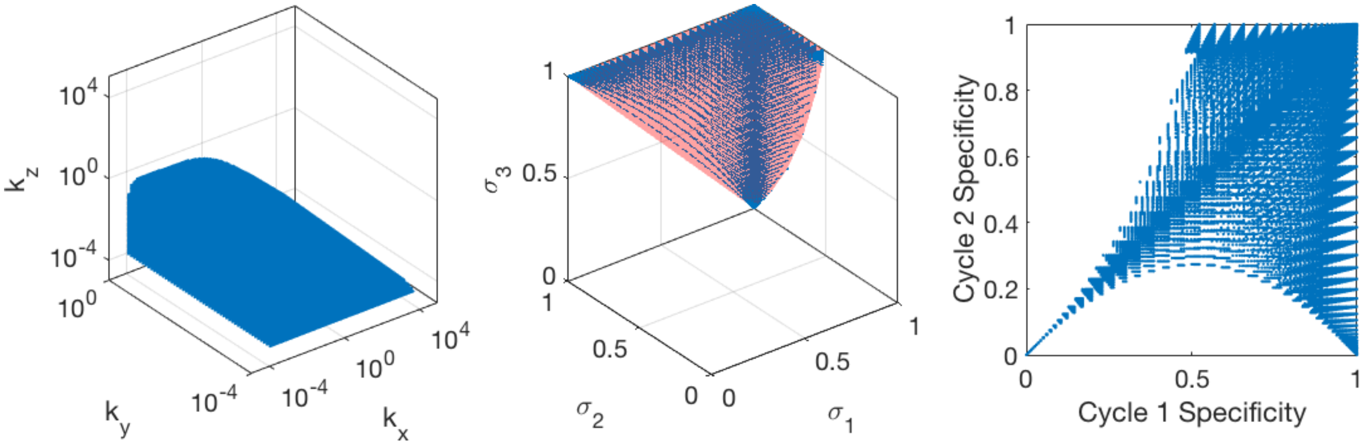


FIG. 3. **Scheme 5:** (a) Scatter plot of $k_{x,y,w}$ values for which real part of at least one eigenvalue is positive. (b) The scatter plot of $\sigma_{1,2,3}$ for which the same condition is true. (c) Scatter plot of cycle specificities of the two coupled cycle for the same condition. Positive eigenvalue is observed even when the cycle specificities are much below 0.5.

## II. PROBABILITY OF SELF-REPLICATION

For successful self-replication, there must be a region in the parameter space, where the driven autocatalytic cycles can proliferate without any interference from parasitic side reactions. Hence, it is helpful to understand the percolation of autocatalytic cycles and the side reactions in our reaction network.

### A. Percolation of autocatalytic cycles with access to food

The percolation of autocatalytic cycles with access to food depends on two factors:

1. Availability of at least one autocatalytic cycle.
2. Availability of high free energy molecules to drive an autocatalytic cycle.

The probability of meeting both of these conditions are dependent on the underlying reaction network. However, a few qualitative features applies to any reaction network in general, which we outline here.

Let's assume there are total $N$ reversible reactions, half of which we designate as forward reactions and rest as reverse. In a pruned reaction network, we sample a reactions from the forward set with probability $p_{fast}$ and include the corresponding reverse reaction as well. Therefore, there are, on average, $n_f = p_{fast}N$ reactions in the pruned reaction network. Let food, $\mathscr{F}$,

be the molecules that are provided in abundance to fuel the chemical reactions. For example, in our model $B$ and $G$ are the fuel or food molecules and they can be used to produce other molecules required for various autocatalytic cycles.

#### 1. Availability of food

Since we select the reactions randomly from the complete set of reactions, it is likely to encounter a situation where there are no mechanisms to utilize $\mathscr{F}$ in the pruned reaction network. Hence, we compute the probability to find a mechanism to generate food from the fuel molecule in the pruned network. To do so, we note that there are two principal mechanisms for such conversion: (a) **direct reactions**, where two fuel molecules react to form a food molecule and (b) **catalytic cycles**, where two or more fuel molecules are converted to food molecules via two or more coupled reactions. Let, $p_d$ be the probability of sampling a direct reaction and $p_c$ be the probability of sampling a catalytic cycle. $p_d$ can be easily approximated from the information about the reactions: if there are $n_d$ direct reactions, then the probability of sampling one of them is $p_d = 2n_d/N$. The factor of 2 appears because either (a) we can choose all of the direct reactions to be forward reaction, in which case we sample $n_d$ reactions from $N/2$ reactions or (b) of we pick their reverse reaction, automatically they are included in the reaction network, hence we sample $2n_d$ reactions from $N$ reactions. Calculating $p_c$ is tougher.

The number of catalytic cycles increases with the number of constituent reactions $m$ for $m << N$. However, a functional catalytic cycles require a steady flow of flux through its constituent reactions to be effective. As pointed out in several studies [King, Szathmary], the likelihood of obtaining such functional cycles decreases exponentially in $m$ for generic reaction networks. Hence, $p_c$ can be well approximated by calculating the likelihood, $p_{c\mathscr{F}}$, of finding a two-step catalytic cycle that converts the fuels into food for the autocatalytic cycles. Generically, the reactions look like the following:

$$\mathscr{F}_1 + \mathscr{C}_1 \rightarrow \mathscr{C}_2 + \mathscr{R}_1 \tag{28}$$

$$\mathscr{F}_2 + \mathscr{C}_2 \rightarrow \mathscr{C}_1 + \mathscr{R}_2 \tag{29}$$

Here, $\mathscr{F}_{1,2}$ are the fuel molecules and they can be identical, $\mathscr{C}_{1,2}$ are intermediate molecules that effectively act like catalysts, and $\mathscr{R}_{1,2}$ are the produced food molecules. The number of all two-step cycles, $N_{C2}$, can be calculated from the adjacency matrix of the reaction network. This number gives the probability of finding a catalytic cycle when two reactions, which are not each others reverse reaction, are chosen randomly:

$$p_{cyc} = \frac{2N_{C2}}{N(N-2)} \tag{30}$$

With the additional information about the reactions that utilize $\mathscr{F}$, the number of such conversion cycles, $n_{c\mathscr{F}}$, can be computed, whence

$$p_{c\mathscr{F}} = n_{c\mathscr{F}}/N_{C2}. \tag{31}$$

With these two probabilities, $p_d$ and $p_{c\mathscr{F}}$, available, we compute the probability of finding at least one mechanism that converts fuel into food. To do so, we first compute the probability of finding at least one direct mechanism:

$$\begin{aligned} p_{d\geq 1} &= 1 - \text{Probability( no direct mechanism )} \\ &= 1 - (1-p_d)^{n_f} \end{aligned} \tag{32}$$

Similarly, probability of finding at least one conversion cycle is:

$$p_{c\mathscr{F}\geq 1} = 1 - \langle (1-p_{c\mathscr{F}})^{n_{C2}} \rangle \leq 1 - (1-p_{c\mathscr{F}})^{\langle n_{C2} \rangle} \tag{33}$$

Here $\langle n_{C2} \rangle = p_{cyc} \times n_f(n_f-2)/2$ is the expected number of cycles in the pruned network. Therefore, probability of finding at least one mechanism of food production is:

$$p_{food} = 1 - (1-p_{d\geq 1})(1-p_{c\geq 1}) \tag{34}$$

$$\tag{35}$$

#### 2. Availability of autocatalytic cycle

Autocatalytic cycles are subsets of catalytic cycle. Hence, finding an autocatalytic cycle is harder than finding a catalytic cycle. Let's assume that there are $n_{ac2}$ two step autocatalytic cycle. Therefore, the probability, that a randomly chosen catalytic cycle is an autocatalytic cycle is:

$$p_{ac2} = n_{ac2}/N_{C2} \tag{36}$$

Therefore, probability of finding at least one autocatalytic cycle is:

$$p_{ac\geq 1} \leq 1-(1-p_{ac2})^{\langle n_{C2}\rangle} \tag{37}$$

Since this inequality provides an upper bound for $p_{ac\geq 1}$, for simplicity of calculation we assume that $p_{ac\geq 1} = 1-(1-p_{ac2})^{\langle n_{C2}\rangle}$. In the same spirit, we assume that $p_{c\mathscr{F}\geq 1} = 1-(1-p_{c\mathscr{F}})^{\langle n_{C2}\rangle}$.

### 3. *Probability of autocatalytic cycles with access to food*

Combining the results from the previous two sections, we find the probability of finding at least one autocatalytic cycle with access to food:

$$p_{acc} = p_{ac\geq 1} \times p_{food} \tag{38}$$

(39)

## B. Probability of side reactions

Let $n_R$ be the average number of reactions that a particular molecule react in and $p_R = n_R/N$ be the average probability that a particular molecule is the reactant in a randomly chosen reaction. Hence, if $n_f$ reactions are chosen randomly then the probability that a molecule reacts in more than one reactions is:

$$p_{r>1} = 1-(1-p_r)^{n_f} - n_f p_r (1-p_r)^{n_f-1} \tag{40}$$

Statistically, as long as there is at least one molecule that reacts in at most one reaction, there will be at least one autocatalytic cycle without any side reactions, which will permit exponential growth. Hence, side reactions start to interfere only when all the molecules take part in more than one reactions. The emergence of the lossy side reactions also depend on whether the dimerization reactions, such as $B+G \rightarrow BG$ and others, are forbidden or not. If one or more of them are forbidden, then the percolation of the lossy side reactions become more difficult than when all of them are allowed. Therefore, the probability of finding all autocatalytic cycles with side reactions is:

$$\begin{aligned} p_{loss} &= \text{Prob(all molecules except fuels react in more than one reactions )} \\ &= p_{r>1}^{N_M - N_{\mathscr{F}}} \times (1-(1-p_d)^{n_f}) \end{aligned} \tag{41}$$

Here $p_d$ is the probability of the dimerization reaction, which is also the probability for the direct access to the food. $N_M$ is the total number of molecules in the reaction network and $N_{\mathscr{F}}$ is the number of fuel molecules.

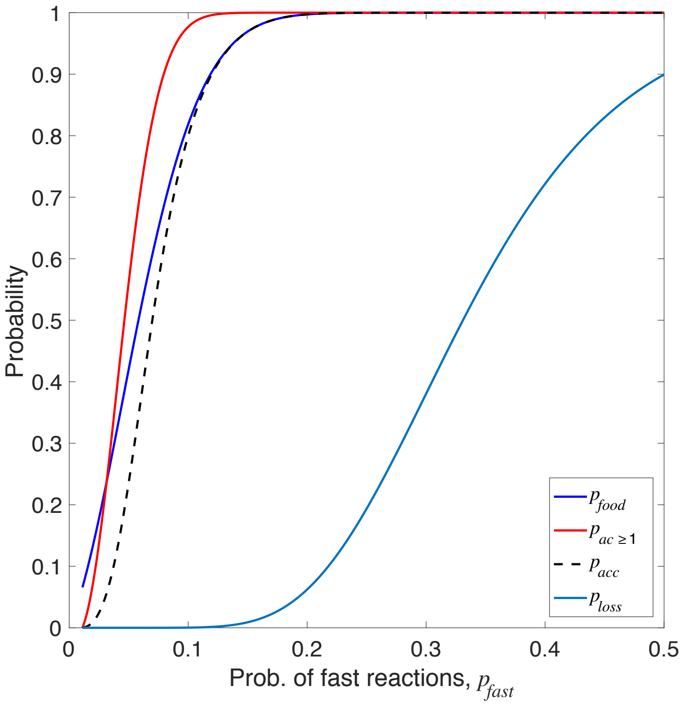


FIG. 4. Percolation of various structures in the used reaction network vs. the probability of fast reactions: Mechanisms that converts fuel into food, $p_{food}$, (blue solid line), Autocatalytic cycles, $p_{ac\geq 1}$, (red solid line), Autocatalytic cycles with access to food, $p_{acc}$, (black broken line) and side reactions, $p_{loss}$ ,(solid gray-blue line).

### C. Probability of self-replication

An autocatalytic cycle runs efficiently if it has direct access to available food and there are no lossy side reactions. Hence, the probability of observing self-replication is:

$$p_{sr} = p_{acc} \times (1 - p_{loss}) \tag{42}$$

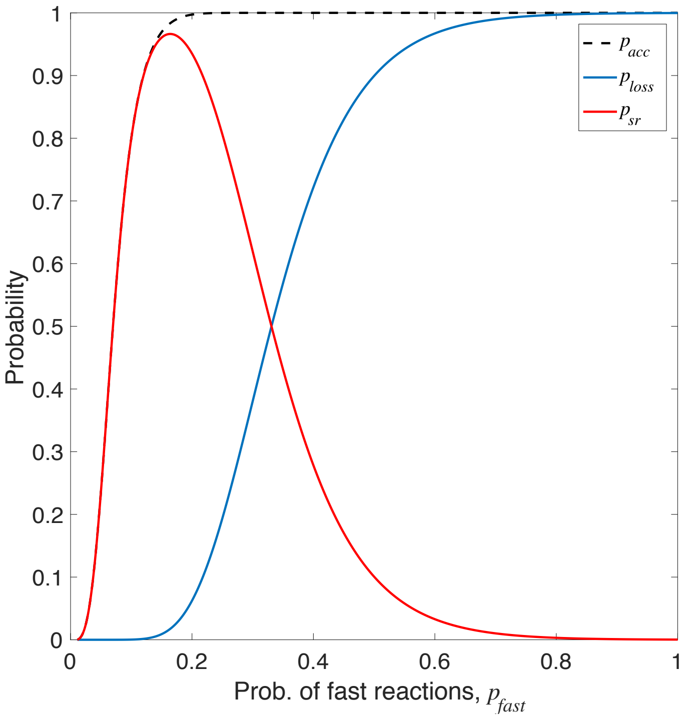


FIG. 5. Probability of self-replication vs. the probability of fast reactions: Prob. of autocatalytic cycles with access to food, $p_{acc}$, (black broken line), side reactions, $p_{loss}$ (solid gray-blue line), and self-replication, $p_{sr}$ (solid red line).

### D. Percolation probabilities and conditions for self-replication

As can be seen in Fig. 4, in the reaction network used in our model, the percolation of autocatalytic cycles with access to food happens at a lower value of $p_{fast}$ than the percolation of lossy side reactions. Hence, for some intermediate values of $p_{fast}$, we obtain a reaction network that is predominantly made of interacting autocatalytic cycles with no side reactions. In that intermediate region, self-replication happens optimally (Fig. 5). It is easy to imagine a reaction network where the opposite happens: $p_{loss}$ percolates before $p_{acc}$. In the intermediate region the network is more tree like and in such a network self-replication is unlikely to happen. Therefore, **in general, if cycle is the predominant structural motif in a reaction network, then it is conducive for self-replication**.

### E. Asymptotic bound on the probability of self-replication

When $N_m \to \infty$ and $p_r \to 0$ $(N \to \infty)$, $p_{loss}$ is a step function and provides a strong upper bound for $p_{fast}$ values that allow self-replication. This upper bound can be calculated by finding the $p_{fast}$ value for which the derivative of $p_{loss}$ with respect to $p_{fast}$ is maximum. Upon calculation, we find that for self-replication to occur:

$$\boxed{p_{fast}^{max} \leq \frac{\log N_m}{N_m}}. \tag{43}$$

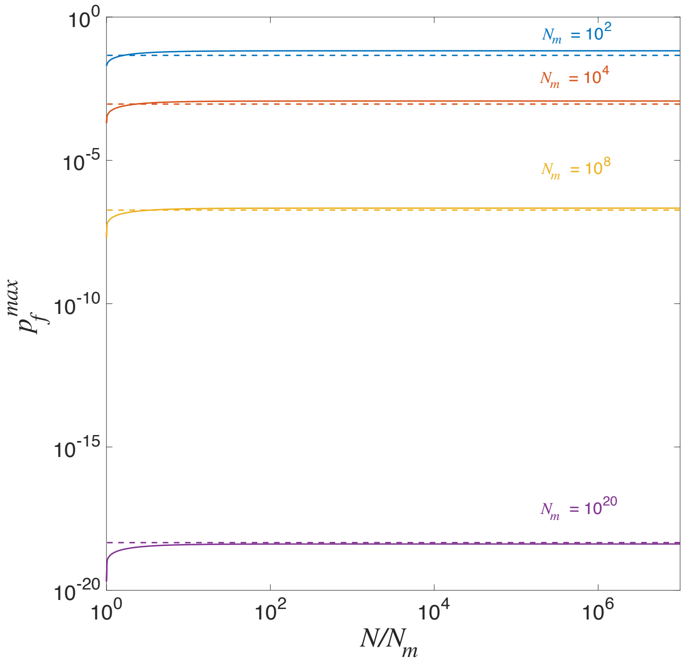


FIG. 6. The position of maximum, $p_{fast}^{max}$ vs. the complexity of the reaction network $N/N_m$. Irrespective of the value of $N_m$, $p_{fast}^{max}$ stays unchanged when the complexity $N/N_m$ is large enough ($\geq 10$) as shown in the numerically calculated curves (solid lines). In the large complexity limit, when $N_m$ is large, $p_{fast}^{max}$ is well approximated by the theoretical bound (broken lines) in Eq. 43.

## III. FACTORS AFFECTING PROBABILITY OF SELF-REPLICATION

It is unlikely that $p_{fast}$, which controls the mean number of nodes in the reaction network, is the only factor that determines the probability of self-replication. In any network, the most important network elements are the number of nodes, number of edges, and number of cycles, which we measure respectively by the number of fast reactions $n_f$, mean degree of the nodes in the reaction network $n_e$, and the number of two cycles in the reaction network $n_{ac2}$. In any graph these three quantities are linearly dependent on each other. Therefore, we have chosen to report the dependence of exponential growth on $p_{fast}$ and $n_e$.

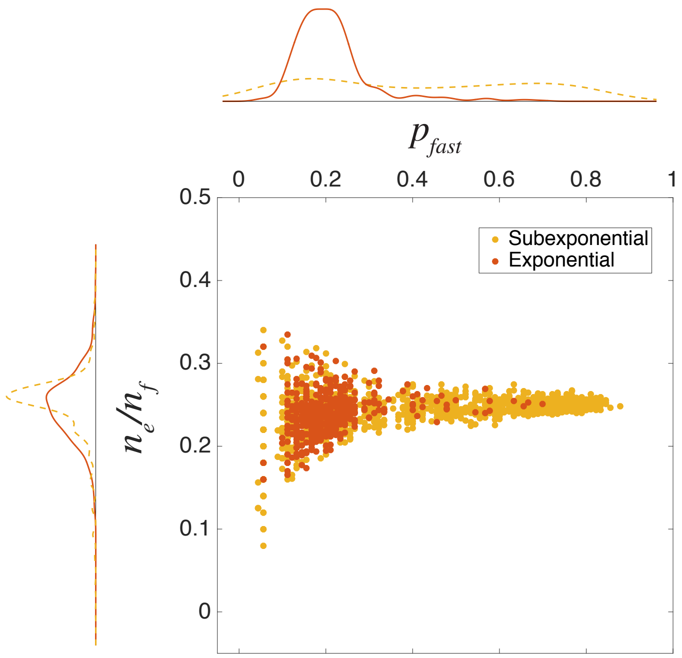


FIG. 7. Scatter plot of mean degree per node, $n_e/n_f$ and $p_{fast}$. The red points correspond to exponential growth and the orange point correspond to subexponential growth. As can be seen from the histogram on the y axis, emergence of exponential growth does not have strong dependence on the mean degree distribution.

## IV. CONTROL OF $p_{sr}$ THROUGH DIMERIZATION REACTIONS

The relation, $p_{sr} = p_acc \times p_loss$, is purely topological, in the sense that both $p_{acc}$ and $p_{loss}$ depends only on the reaction network properties. Therefore, by controlling these properties, such as the density of autocatalytic cycles, the degree distribution, or the number of reactions, it is possible to control the range of $p_{fast}$, over which $p_{sr}$ remains reasonably high. The density of the autocatalytic cycles is difficult to control independently since in a strongly interacting network, such as ours, they are too numerous and interdependent, which renders the control of $p_{acc}$ nearly impossible. On the other hand, there is a simple way to control $p_{loss}$. The lossy side reactions overwhelm the autocatalytic cycle if the reaction network is sufficiently "well-connected", i.e., if it is possible to generate all the molecules by seeding the reaction network with the atoms ($B$ and $G$) only. Therefore, the dimerization reactions – the reactions that convert the atoms to their dimers – are necessary to construct a well-connected reaction network and, hence, the percolation of the lossy side reactions. Consequently, by manipulating the rate of the dimerization reactions, the percolation of $p_{loss}$ can be manipulated. As we show in Fig. 8, rendering one or more dimerization reactions always forbidden improves the probability of self-replication. In fact, when all three of them are always forbidden, for large $p_{fast}$, self-replication occurs with unit probability. The propensity of the dimerization reactions determine the stability of the food molecules, $B$ and $G$. Therefore, in general, this result implies that the more stable the food molecule, the more likely it is to attain exponential growth.

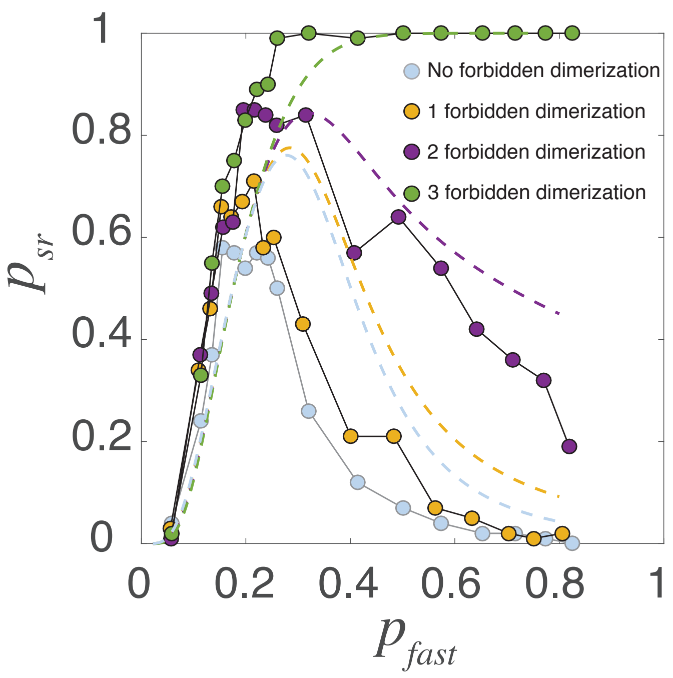


FIG. 8. Probability of self-replication vs. the probability of fast reactions with different numbers of forbidden dimerization reactions. Increasing the number of forbidden dimerization reactions increase the stability of the food molecules $B$ and $G$, and the probability of self-replication increases.

## V. PROBABILITY DISTRIBUTION FOR SPECIFICITY

Let's assume that the propensities (rates), $x$, are distributed according to a probability distribution function $\rho_p(x)$. Let's further assume that every reaction competes, on average, with $C$ other reactions. In reality, each reaction competes with varying number of reactions, but for this example, we ignore that complication. Furthermore, let's assume that these reactions, on average, have propensities $\mu$, which is the mean propensity. Therefore, on an average, a reaction with propensity $x$ will have specificity:

$$\sigma = \frac{x}{x + C\mu} \tag{44}$$

The probability distribution for $\sigma$ is then obtained by change of variables:

$$\rho_s(\sigma)d\sigma = \rho_p(x)dx \tag{45}$$

$$\therefore, \rho_s(\sigma) = \rho_p\left(\frac{C\mu\sigma}{1-\sigma}\right) \times \frac{(1-\sigma)^2}{C\mu} \tag{46}$$

$$\tag{47}$$

For exponentially distributed propensities, $\rho_p(x) = \lambda \exp(-\lambda x)$, where $\mu = 1/\lambda$:

$$\rho_s\sigma = \frac{\lambda^2}{C}(1-\sigma)^2 \exp\left(-\frac{C\sigma}{1-\sigma}\right) \tag{48}$$

For power law distributed propensities with exponential cutoff $\rho_p(x) \sim x^\nu \exp(-\lambda x)$, where $\mu = \frac{\nu+1}{\lambda}$:

$$\rho_s(\sigma) \sim \left(\frac{\Gamma(\nu+1)}{\lambda^{\nu+1}}\right)^{\nu+1} \left(\frac{C\sigma}{1-\sigma}\right)^\nu \exp\left(-\frac{\Gamma(\nu+1)}{\lambda^{\nu+1}} \frac{C\lambda\sigma}{1-\sigma}\right) \tag{49}$$

[1] E. Szathmáry, "The origin of replicators and reproducers," Philosophical Transactions of the Royal Society B: Biological Sciences **361**, 1761–1776 (2006).
[2] G. King, "Recycling, reproduction, and life's origins," Biosystems **15**, 89–97 (1982).
